# Supplementary material for: Analytical mesoscale modeling of aeolian sand transport
Source: arXiv:1405.0624 ancillary file (2017-09-04)
Supplement: Supplementary file 1 [file supplementary_material.pdf]

# Mesoscale Modeling of Aeolian Sand Transport

## Supplementary Material

Marc Lämmel, Anne Meiwald, and Klaus Kroy

*Institut für theoretische Physik, Universität Leipzig, Postfach 100920, 04009 Leipzig, Germany*

(Dated: May 3, 2014)

We present a criterion for estimating the mean vertical ejection speed  $v_{z0}^{\text{rep}}$ , compare the tow-species prediction of  $v_{\text{sal},z0}/v_{\text{sal}}$  to several collision experiments, investigate the influence of the shape of the saltation flux profile on the mean transport layer height  $z_m$ , and estimate the minimal dune size  $L_{\text{min}}$  from a linear stability analysis.

### S1. REPTATION VELOCITY $v_{z0}^{\text{rep}}$

In the two-species formalism [1], saltions and reptons are two effective representative species, loosely corresponding to the common phenomenological classification: saltions do and reptons do not cause a splash; reptons are moreover shielded from the actual wind conditions by the saltions, under stationary transport conditions, a feature commonly known under the name of “Bagnold focus”. It renders the kinematics of the reptons essentially independent of the actual wind strength during stationary saltation. From these two characterizations of the reptons, one obtains upper bounds for  $v_{z0}^{\text{rep}}$ . To fix the numerical value, required in the main text, we draw upon the collision experiments by Beladjine *et al.* [6]. They suggest  $v_{z0}^{\text{rep}} \approx 4(gd)^{1/2} \approx u_{*t}$ , considerably below the minimum speed for splashing, and corresponding to a jump height about one third of the height of the Bagnold focus (cf. Fig. 2 of Ref. [1]).

### S2. REBOUND EFFICIENCY $v_{z0}^{\text{sal}}/v_{\text{sal}}$

In Figs. 2, 3, and 4 of the main text, we compare the two-species result for the hop length and the transport layer height to experimental data, using the ratio  $v_{z0}^{\text{sal}}/v_{\text{sal}}$  as a free fit parameter. In the following, we test if the fit values are consistent with the model, by estimating them from the (effective) restitution coefficient

$$\alpha = v_{z0}^{\text{sal}}/(v_{xi}^{\text{sal}} - v_{x0}^{\text{sal}}) \quad (\text{S1})$$

that is usually employed as the corresponding phenomenological fit parameter in the two-species model [1] ( $v_{xi}^{\text{sal}}$  is the horizontal impact,  $v_{x0}^{\text{sal}}$  the horizontal rebound velocity). To this end, we have to reduce the number of unknown variables, because only  $v^{\text{sal}}$  and  $\alpha$  are determined in the two-species model, while  $v_{z0}^{\text{sal}}$ ,  $v_{xi}^{\text{sal}}$ , and  $v_{x0}^{\text{sal}}$  are unconstrained. We estimate the trajectory of a saltion by numerically integrating the equations of motion

$$\dot{v}_x^{\text{sal}} = \frac{g}{(v_{\infty}^{\text{sal}})^2} |u - v_x^{\text{sal}}| (u - v_x^{\text{sal}}) \quad \text{and} \quad \dot{v}_z^{\text{sal}} = -g, \quad (\text{S2})$$

with the initial values  $v_x^{\text{sal}}(t=0) = v_{x0}^{\text{sal}}$  and  $v_y(t=0) = v_{z0}^{\text{sal}}$  provided by the rebound velocities. Explicit

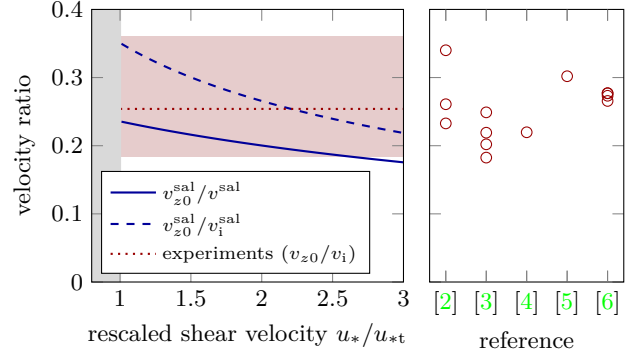

FIG. S1. The velocity ratios  $v_{z0}^{\text{sal}}/v_{\text{sal}}$  and  $v_{z0}^{\text{sal}}/v_i^{\text{sal}}$  as obtained from the tow-species model by numerically integrating the equations of motion for a saltion, Eq. (S2). The grain size was set to  $250\mu\text{m}$  to compare the result for  $v_{z0}^{\text{sal}}/v_i^{\text{sal}}$  with various collision experiments [2–6] shown in the right panel. These data yield a mean vertical rebound–impact velocity ratio  $v_{z0}/v_i \approx 0.25$  and range from 0.18 to 0.34 (shaded area in the left panel).

expressions for the terminal velocity  $v_{\infty}^{\text{sal}}$  and the wind profile  $u \equiv u[z(t)]$  appearing in Eq. (S2) are given by Eqs. (C.2) and (21) of Ref. [1], respectively. From the solution  $\{v_x^{\text{sal}}(t), v_z^{\text{sal}}(t)\}$  we compute the mean vertical grain speed, identified with  $v^{\text{sal}}$ ,

$$v^{\text{sal}} = (t^{\text{sal}})^{-1} \int_0^{t^{\text{sal}}} dt v_x^{\text{sal}} \quad (\text{S3})$$

and the horizontal impact

$$v_{xi}^{\text{sal}} = v_x(t^{\text{sal}}). \quad (\text{S4})$$

Given the two-species quantities  $\alpha$  and  $v^{\text{sal}}$ , the three Eqs. (S1), (S3), and (S4) can be readily solved for  $v_{z0}^{\text{sal}}$ . This procedure yields a weakly  $u_*$ -dependent  $v_{z0}^{\text{sal}}/v^{\text{sal}}$  of size 0.23 for  $u_* \approx u_{*t}$ , as shown in the left panel of Fig. S1.

To make contact with results from collision experiments, we note that these studies provide a relation between the rebound speed  $v_{z0}^{\text{sal}}$  and the impact speed  $v_i^{\text{sal}}$ . We therefore compute

$$(v_i^{\text{sal}})^2 = \left[ \frac{1}{t^{\text{sal}}} \int dt v_x^{\text{sal}}(t) \right]^2 + \left[ \frac{1}{t^{\text{sal}}} \int dt v_z^{\text{sal}}(t) \right]^2 \quad (\text{S5})$$

numerically from the saltation trajectories as described above. The ratio  $v_{z0}^{\text{sal}}/v_i^{\text{sal}}$  is then found to attain values in a rather narrow range 0.2–0.35 (left panel of Fig. S1), which is indeed in good agreement with the collision data published in Refs. [2–6] (right panel of Fig. S1) that yield a mean value of 0.25 for this velocity ratio.

The good agreement between the two-species predictions and the collision experiments shown in Fig. S1 gives strong evidence that the numerically solved scheme proposed above, and thus the resulting value  $v_{z0}^{\text{sal}}/v^{\text{sal}} \approx 0.23$  for  $\tau \approx \tau_t$ , reliably describe the rebound of the saltating grains.

### S3. MEAN TRANSPORT LAYER HEIGHT $z_m$

To compute the mean height  $z_m$  of the saltation layer, defined in Eq. (2) and shown in Figs. 3 and 4 of the main text, we employed a simple exponential distribution for the saltation flux profile  $\partial_z q^{\text{sal}}(z)$ . Here, we investigate the influence of the specific form of this profile on the obtained value of  $z_m$ , replacing the exponential by a log-normal, a truncated power law, and a single trajectory profile.

We write the flux profile  $\partial_z q^{\text{sal}}(z)$  in terms of a scaling function  $f(\zeta) \equiv h^{\text{sal}} \partial_z q^{\text{sal}}(\zeta h^{\text{sal}})/q^{\text{sal}}$  using the mean hop height  $h^{\text{sal}} = (v_{z0}^{\text{sal}})^2/(2g)$  of the saltating grains. (Note that  $f(\zeta)$  is normalized, i.e.,  $\int_0^\infty d\zeta f(\zeta) = 1$ .) Then, Eq. (2) reads

$$1 - q^{\text{rep}}/q^{\text{sal}} = 2 \int_0^{z_m/h^{\text{sal}}} d\zeta f(\zeta). \quad (\text{S6})$$

Substituting the log-normal distribution  $f(\zeta) = \exp[-(\sigma^2/2 + \ln \zeta)^2/(2\sigma^2)]/(\sqrt{2\pi}\sigma\zeta)$  into Eq. (S6), we obtain

$$z_m/h^{\text{sal}} = \exp \left[ -\sigma^2/2 - \sqrt{2}\sigma \text{erf}^{-1}(q^{\text{rep}}/q^{\text{sal}}) \right], \quad (\text{S7})$$

while a truncated power law of the form  $f(\zeta) = (1 + \nu)\zeta_{\text{co}}^{-1-\nu}\zeta^\nu$  with cut-off height  $\zeta_{\text{co}}$  and  $-1 < \nu < 0$ , yields

$$z_m/h^{\text{sal}} = 2^{-1/(1+\nu)}\zeta_{\text{co}}(1 - q^{\text{rep}}/q^{\text{sal}})^{1/(1+\nu)}. \quad (\text{S8})$$

We can also utilize the single trajectory representation for the saltating grain fraction to derive a saltation flux profile from the time interval  $dt$  the salton needs to cross a horizontal slice of thickness  $dz$  at height  $z$ . Neglecting vertical drag forces, the total hop time can be approximated by  $2v_{z0}^{\text{sal}}/g$ , and the probability to find the salton at height  $z$  is obtained as  $\partial_z \rho^{\text{sal}}(z)dz/\rho = gdt/(2v_{z0}^{\text{sal}})$ , which yields

$$2h^{\text{sal}}\partial_z \rho^{\text{sal}}(z)/\rho = (1 - z/h^{\text{sal}})^{-1/2}. \quad (\text{S9})$$

The right-hand side is derived from the vertical speed  $|dz/dt| = [(v_{z0}^{\text{sal}})^2 - 2gz]^{1/2}$ , with which each grain crosses the height  $z$  both on the ascending and on the descending part of its trajectory. To get from Eq. (S9) to the

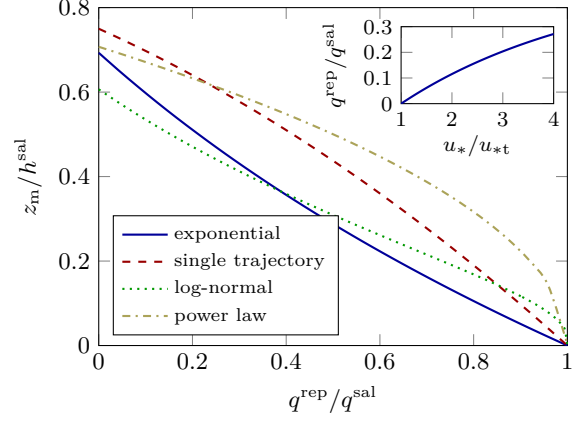

FIG. S2. The mean transport layer height  $z_m$  (rescaled by the saltans' mean hop height  $h^{\text{sal}}$ ) versus the flux ratio  $q^{\text{rep}}/q^{\text{sal}}$  for various flux profiles  $f(\zeta)$  of the saltating grain fraction. The exponential profile used in the main text is compared to the log-normal, given by Eq. (S7), and a power-law distribution, Eq. (S8). We also added the result of the single trajectory approach, Eq. (S10), where the  $z$ -dependence is solely due to the varying time span a salton needs to cross a horizontal layer at height  $z$ . The inset shows the wind strength dependence of the flux ratio  $q^{\text{rep}}/q^{\text{sal}}$  as obtained from the two-species model with the parameters used in the main text.

flux profile  $\partial_z q^{\text{sal}}(z)$  requires an estimate for the horizontal grain speed  $v^{\text{sal}}(z)$  at the height  $z$ , averaged over these two parts of the trajectory. It depends only weakly on  $z$ , as seen by numerically integrating the equations of motions for a hopping grain, as explained in Sec. S2. Approximating the grain velocity  $v^{\text{sal}}(z)$  by its height-averaged value  $v^{\text{sal}}$ , we can thus estimate the flux profile  $\partial_z q(z) \approx v^{\text{sal}} \partial_z \rho^{\text{sal}}(z)$  from Eq. (S9) and obtain the scaling function  $f(\zeta) = (1/2)(1 - \zeta)^{-1/2}$ , for which Eq. (S6) is readily integrated. This yields the mean saltation layer height

$$z_m/h^{\text{sal}} = (1 - q^{\text{rep}}/q^{\text{sal}})(3 + q^{\text{rep}}/q^{\text{sal}})/4. \quad (\text{S10})$$

As illustrated in Fig. S2, we found that all profiles result in qualitatively similar heights  $z_m(q^{\text{rep}}/q^{\text{sal}})$  as function of the flux ratio  $q^{\text{rep}}/q^{\text{sal}}$  and conclude that the shape of  $z_m(u_*)$  shown in Fig. 3 is reasonably independent of the exact form of  $f(\zeta)$ . The differences between the curves in Fig. S2 would weakly alter the value of the fit parameter  $v_{z0}^{\text{sal}}/v^{\text{sal}}$  to match the experimental data for  $z_m$  in Figs. 3 and 4, but are otherwise not significant. This justifies the use of the exponential distribution in the main text as the simplest representation of the saltation flux profile.

### S4. MINIMAL DUNE SIZE $L_{\text{min}}$

In this section, we estimate the minimal dune length  $L_{\text{min}}$ , shown in Fig. 5, from a linear stability analysis of the evolution of a weakly perturbed flat bed. This analysis was first proposed by Andreotti *et al.* [7]; and

its most recent version can be found in Ref. [8], which provides the basis for the following derivation of  $L_{\min}$ . In fact, we present a slightly improved version of the original argument, which yields a qualitatively different result for the ratio  $L_{\min}/\ell_{\text{sat}}^{\text{dune}}$ .

The linear stability analysis is based on the (out of phase) response of shear stress and sand transport to weak perturbations of a flat bed [9, 10]. It allows to calculate the wavelength of the (initially) fastest growing mode of the profile, which is identified with  $L_{\min}$ . In Ref. [8], Andreotti and coworkers used the generic formula  $q_{\text{sat}} \propto \tau^\gamma(\tau - \tau_t)$  for the saturated flux, which is indirectly slope-dependent via the local shear stress  $\tau$  and via the threshold value  $\tau_t$ . However, they neglected the direct slope dependence, which should be accounted for to first order in  $h'$  according to

$$q_{\text{sat}} \propto \tau^\gamma(\tau - \tau_t)(1 - h' \cot \theta_f), \quad (\text{S11})$$

where  $\theta_f$  is the friction angle. This direct slope dependence of  $q_{\text{sat}}$  was first predicted by Bagnold and later validated by Iversen and Rasmussen [11], who obtained  $\theta_f \approx 40^\circ$  for typical sand (with grain diameter  $d \geq 170 \mu\text{m}$ ). Eq. (S11) can also be derived from the continuum saltation model by Sauermann *et al.* [12] if we extend its kinematics to sloped beds. Accounting for the gravitational force  $-gh'$  in the momentum balance, Eq. (33) in Ref. [12], we obtain

$$q_{\text{sat}} \propto v_0(\tau - \tau_t)(1 - h' \alpha v_\infty / v_0). \quad (\text{S12})$$

Here, the terminal velocity  $v_\infty$  accounts for the bed friction and is equal to the difference between the wind speed and the steady-state transport velocity  $v_0$  over the unperturbed bed. For moderate wind strengths, i.e.,  $\tau \approx \tau_t$ ,  $v_0$  is independent of  $\tau$ , corresponding to  $\gamma = 0$ , and the coefficient  $\alpha v_\infty / v_0$  takes values on the order of 0.5 for typical dune sand, which corresponds to  $\theta_f \approx 60^\circ$  in Eq. (S11). While this numerical value is 3/2 times bigger than the experimentally obtained friction angle, the overall agreement of the derived result with the phenomenological law is reassuring. Moreover, within the improved formalism, one actually should replace the term  $\alpha v_\infty / v_0$  in Eq. (S12) by a weighted average over the saltation and a reptation contribution. If we assume that the friction angle for the reptons is on the order of the sand's dynamic angle of repose, which is about  $34^\circ$ , the mean effective friction angle  $\theta_f$  indeed takes values between  $34^\circ$  and  $60^\circ$ , depending on the precise conditions (chiefly the mass balance of reptons and saltons).

For the stability analysis, we follow Fourrière *et al.* [8] and expand the perturbation  $\delta q_{\text{sat}} = q_{\text{sat}} - q_{\text{sat}0}$  of the saturated flux from its flat bed value  $q_{\text{sat}0}$  to first order in the perturbation  $\delta h$  of the bed profile. From Eq. (S11), we obtain its Fourier transform  $\widehat{\delta q}_{\text{sat}} = \int dx \delta q_{\text{sat}} e^{-ikx} \propto \tau_0^\gamma (a + ib)k \widehat{\delta h}$  with

$$\begin{aligned} a &= A + \gamma A(1 - \tau_{t0}/\tau_0) \quad \text{and} \\ b &= B + \gamma B(1 - \tau_{t0}/\tau_0) - \cot \theta_f, \end{aligned} \quad (\text{S13})$$

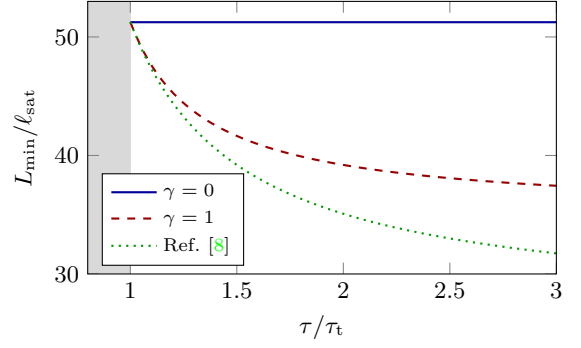

FIG. S3. The ratio  $L_{\min}/\ell_{\text{sat}}^{\text{dune}}$  of the wavelength of the fastest growing mode and the saturation length *versus* wind strength  $\tau/\tau_t$  as obtained from the linear stability analysis proposed in Ref. [8], Eq. (S14), with a directly slope-dependent flux given by Eq. (S11) with the generally accepted exponent  $\gamma = 0$  (solid line) and the (unphysical) exponent  $\gamma = 1$  (dashed). We also added the result of Fourrière *et al.* [8], who neglected the direct slope dependence of  $q_{\text{sat}} \propto \tau - \tau_t$  (dotted line). We used the coefficients  $A = 7$  and  $B = 2.5$  (corresponding to the estimate of Refs. [10, 13] with a hydrodynamic roughness  $\eta_0 = 10^{-3}$ ) and the friction angle  $\theta_f = 40^\circ$  for all three curves.

where we used the shear stress perturbation  $\widehat{\delta \tau}/\tau_0 = (A + iB)k$  (for  $k \geq 0$ ) and the slope-dependent threshold  $\widehat{\delta \tau}_t = ik \widehat{\delta h} \cot \theta_f$ . Only the  $\tau$ -independent term  $\cot \theta_f$  in the expression for  $b$  differs from the result  $(\tau_t/\tau) \cot \theta_f$  by Fourrière *et al.*, who neglected the direct slope dependence of  $q_{\text{sat}}$ . Using the linearized differential equation for the flux evolution and mass conservation, one obtains the ratio  $L_{\min}/\ell_{\text{sat}}^{\text{dune}}$  of the wavelength of the fastest growing mode and the saturation length as a function of the ratio  $a/b$ . With  $L_{\min}/\ell_{\text{sat}}^{\text{dune}} \gg 1$ , this result reads

$$L_{\min}/\ell_{\text{sat}}^{\text{dune}} \approx 3\pi a/b. \quad (\text{S14})$$

Substituting  $a$  and  $b$  from Eq. (S13), we see that  $L_{\min}/\ell_{\text{sat}}^{\text{dune}}$  decreases with increasing  $\tau$  as long as  $\gamma > 0$ . This is qualitatively similar to what was obtained by Fourrière *et al.* neglecting the experimentally well established and theoretically derived rightmost factor in Eq. (S11), as illustrated in Fig. S3. However, for the generally accepted value  $\gamma = 0$  (see also Fig. 1 of the main text), the ratio  $a/b = A/(B - \cot \theta_f)$  becomes independent of  $\tau$ , and so does  $L_{\min}/\ell_{\text{sat}}^{\text{dune}}$ . Evidently, the slope dependence, represented by the angle of repose  $\theta_f$ , leads to a renormalization of the asymmetric part of the flow field perturbation, represented by  $B$ . This correction crucially affects the absolute value of  $a/b = A/(B - \cot \theta_f)$ , because it diverges if  $B$  approaches  $\cot \theta_f \approx 1.2$ , which is indeed within the typical range of  $B$ . The actual values of the coefficients  $A$  and  $B$  can be estimated as functions of the dimensionless hydrodynamic bed roughness  $\eta_0$ . Using the dependencies  $A(\eta_0)$  and  $B(\eta_0)$  proposed by Jackson and Hunt [13], see Ref. [10], we obtain that  $a/b$  diverges at  $\eta_0 \approx 1.7 \times 10^{-5}$ , which is below the lower limit of the estimated range  $10^{-4}$  to  $10^{-2}$  [8] of  $\eta_0$  for typical

sand dunes. We can match the fit result  $L_{\min}/\ell_{\text{sat}}^{\text{dune}} \approx 27$  of Fig. 5 for  $\eta_0 \approx 1.2 \times 10^{-2}$ , at the upper limit of the estimated range.

In summary, we showed that an improved version of the linear stability analysis proposed by Fourrière *et al.* yields a  $\tau$ -independent ratio  $L_{\min}/\ell_{\text{sat}}^{\text{dune}}$ , when the employed stationary flux law is of the, both experimentally and theoretically, well established form given by Eq. (S11) with  $\gamma = 0$ . This is in contrast to the

rapidly decaying  $L_{\min}/\ell_{\text{sat}}^{\text{dune}}$  with increasing  $\tau$  proposed by Fourrière *et al.*, see also Ref. [14]. The absolute value of  $L_{\min}/\ell_{\text{sat}}^{\text{dune}}$  may vary over orders of magnitude. But, its  $\tau$ -independence, together with the experimentally observed wind dependence of the minimal dune size  $L_{\min}$  (see Fig. 5), would implicate that the saturation length  $\ell_{\text{sat}}^{\text{dune}} \propto L_{\min}$  must strongly decrease with increasing wind strength, as indeed predicted by the grain-scale model developed in Ref.[9] and its refined version given in the main text.

- 
- [1] M. Lämmel, D. Rings, and K. Kroy, *New J. Phys.* **14**, 093037 (2012).
  - [2] B. Willetts and M. Rice, *Acta Mech.* **63**, 255 (1986), 10.1007/BF01182552.
  - [3] S. Mitha, M. Tran, B. Werner, and P. Haff, *Acta Mech.* **63**, 267 (1986), 10.1007/BF01182553.
  - [4] B. Werner, *the Journal of Geology*, 1 (1990).
  - [5] F. Rioual, A. Valance, and D. Bideau, *Phys. Rev. E* **62**, 2450 (2000).
  - [6] D. Beladjine, M. Ammi, L. Oger, and A. Valance, *Phys. Rev. E* **75**, 061305 (2007).
  - [7] B. Andreotti, P. Claudin, and S. Douady, *Europ. Phys. J. B* **28**, 341 (2002).
  - [8] A. Fourrière, P. Claudin, and B. Andreotti, *J. Fluid Mech.* **649**, 287 (2010).
  - [9] K. Kroy, G. Sauermann, and H. J. Herrmann, *Phys. Rev. Lett.* **88**, 054301 (2002).
  - [10] K. Kroy, G. Sauermann, and H. J. Herrmann, *Physical Review E* **66**, 1 (2002).
  - [11] J. D. Iversen and K. R. Rasmussen, *Sedimentology* **46**, 4, 723 (1999).
  - [12] G. Sauermann, K. Kroy, and H. J. Herrmann, *Phys. Rev. E* **64**, 031305 (2001).
  - [13] P. S. Jackson and J. C. R. Hunt, *Quart. J. Roy. Meteor. Soc.* **101**, 929 (1975).
  - [14] B. Andreotti, P. Claudin, and O. Pouliquen, *Geomorphology* **123**, 343 (2010).
